# Supplementary material for: Understanding the AI-powered Binary Code Similarity Detection
Source: arXiv:2410.07537 source file (2024-10-10)
Supplement: Supplementary file 1 [file appendix.tex]

\appendix

% \section{}
\section{Appendix}
\label{s:appendix}

\subsection{Mainstream Embedding Neural Networks}
\label{appendix-network-intro}
{\bf NLP-based models.} 
After binary code disassembling, a binary code snippet can be represented using an assembly language, which to some extent shares many analogical topics with a natural language---both of them are organized by specific grammatical structures and can express certain semantics. Therefore, when embedding the obtained instruction sequences, many studies propose to treat instructions as words, functions as sentences, and the whole binaries as paragraphs in natural language. Then, researchers turn to converting the assembly language into low-dimensional vectors in the same way as NLP tasks. For instance, Asm2Vec~\cite{ding2019asm2vec} uses an improved PV-DM model~\cite{le2014distributed}, an unsupervised NLP learning approach, to generate code embedding for binary functions. 

%\item
{\bf RNN/LSTM-based models.} 
Recursive Neural Networks (RNN) and LSTM (a special RNN with gate mechanisms)~\cite{Greff2017LSTM} have been proven to be effective in sentiment analysis, language translation, and question answering. Thus, many studies turn to applying RNN/LSTM models to extract the semantics of binary code. For instance, \textsc{InnerEye}~\cite{zuo2019neural} proposes to use neural machine translation (NMT), a kind of LSTM model, to detect basic block similarity. Asteria~\cite{yang2021asteria} and SAFE~\cite{massarelli2018safe} use LSTM/RNN  to learn the semantic representation of a binary function. 

%\item
{\bf CNN-based models.} 
CNN~\cite{albawi2017understanding} has been widely applied to image and video recognition, classification, and processing, which is good at grasping node connectivity patterns in matrix data through kernels. Considering (1) the raw bytes contain all the semantics of binary code, and (2) the node order of the CFGs of binaries (adjacent matrices) compiled from the same source code is highly likely to remain the same, researchers proposed to learn the raw bytes pattern or the \textit{node order information} of CFGs by CNN, which can be used as an important program feature in binary code similarity detection. For example, BinaryAI~\cite{yu2020order} uses a 3-layer CNN to construct an order-aware model to learn function embedding. $\alpha$Diff~\cite{liu2018alphadiff} represents the raw bytes of binary code as a matrix and then uses a CNN to generate function embeddings. 
 
%\item
{\bf GNN-based models.} 
%Recently, there has been a surge of interest in neural graph networks (GNN), a powerful class of deep learning models that yield effective representation for structured objects. Various of GNNs have been proposed for learning effective graph embedding vectors. 
Using disassembling tools such as IDA~\cite{ida-pro-7-0} and Radare2~\cite{radare2}, one can obtain the graph representation (CFG or DFG) of a binary code snippet. Thus, many \BCSD approaches~\cite{xu2017neural,gao2018vulseeker,Baldoni2018Unsupervised} consider using various kinds of GNNs (a powerful class of deep learning models that yield effective representation for structured objects), including Structure2Vec~\cite{dai2016discriminative}, graph attention networks~\cite{velivckovic2017graph} and graph convolution networks (GCN)~\cite{kipf2016semi, kim2022improving,luovulhawk} to learn the vector representation of binary code. For instance, Gemini~\cite{xu2017neural} improves Genius~\cite{feng2016scalable} by using Structure2Vec~\cite{dai2016discriminative} to transform binary functions into embeddings according to the corresponding CFG and manually extracted features. 
%By leveraging both the CFG and DFG, Vulseeker~\cite{gao2018vulseeker} and Vulseeker-pro develops a deep neural network (DNN) model to extract the graph embedding vector, which can be used to represent the entire binary function semantics. 

%\item
{\bf Other models.} 
Except for the above mainstream neural networks, other neural networks such as message-passing neural networks (MPNN)~\cite{gilmer2017neural} and proc2vec~\cite{shalev2018binary} are also applied to the existing AI-power \BCSD tools. For instance, BinaryAI~\cite{yu2020order} also adopts MPNN, which extracts the structural information of a binary CFG to learn the representation of binary code. In this paper, we aim to comprehensively evaluate the widely used embedding neural networks, including the NLP-based, RNN/LSTM-based,  CNN-based, and GNN-based models.

\begin{figure*}[htbp]
    \begin{minipage}[t]{1\textwidth}
        \centering
            \subfloat[rawbyte_difference-x64]{
                    \label{same-arch-rawbyte-distribution-x64} 
                    \includegraphics[width=0.24\textwidth]{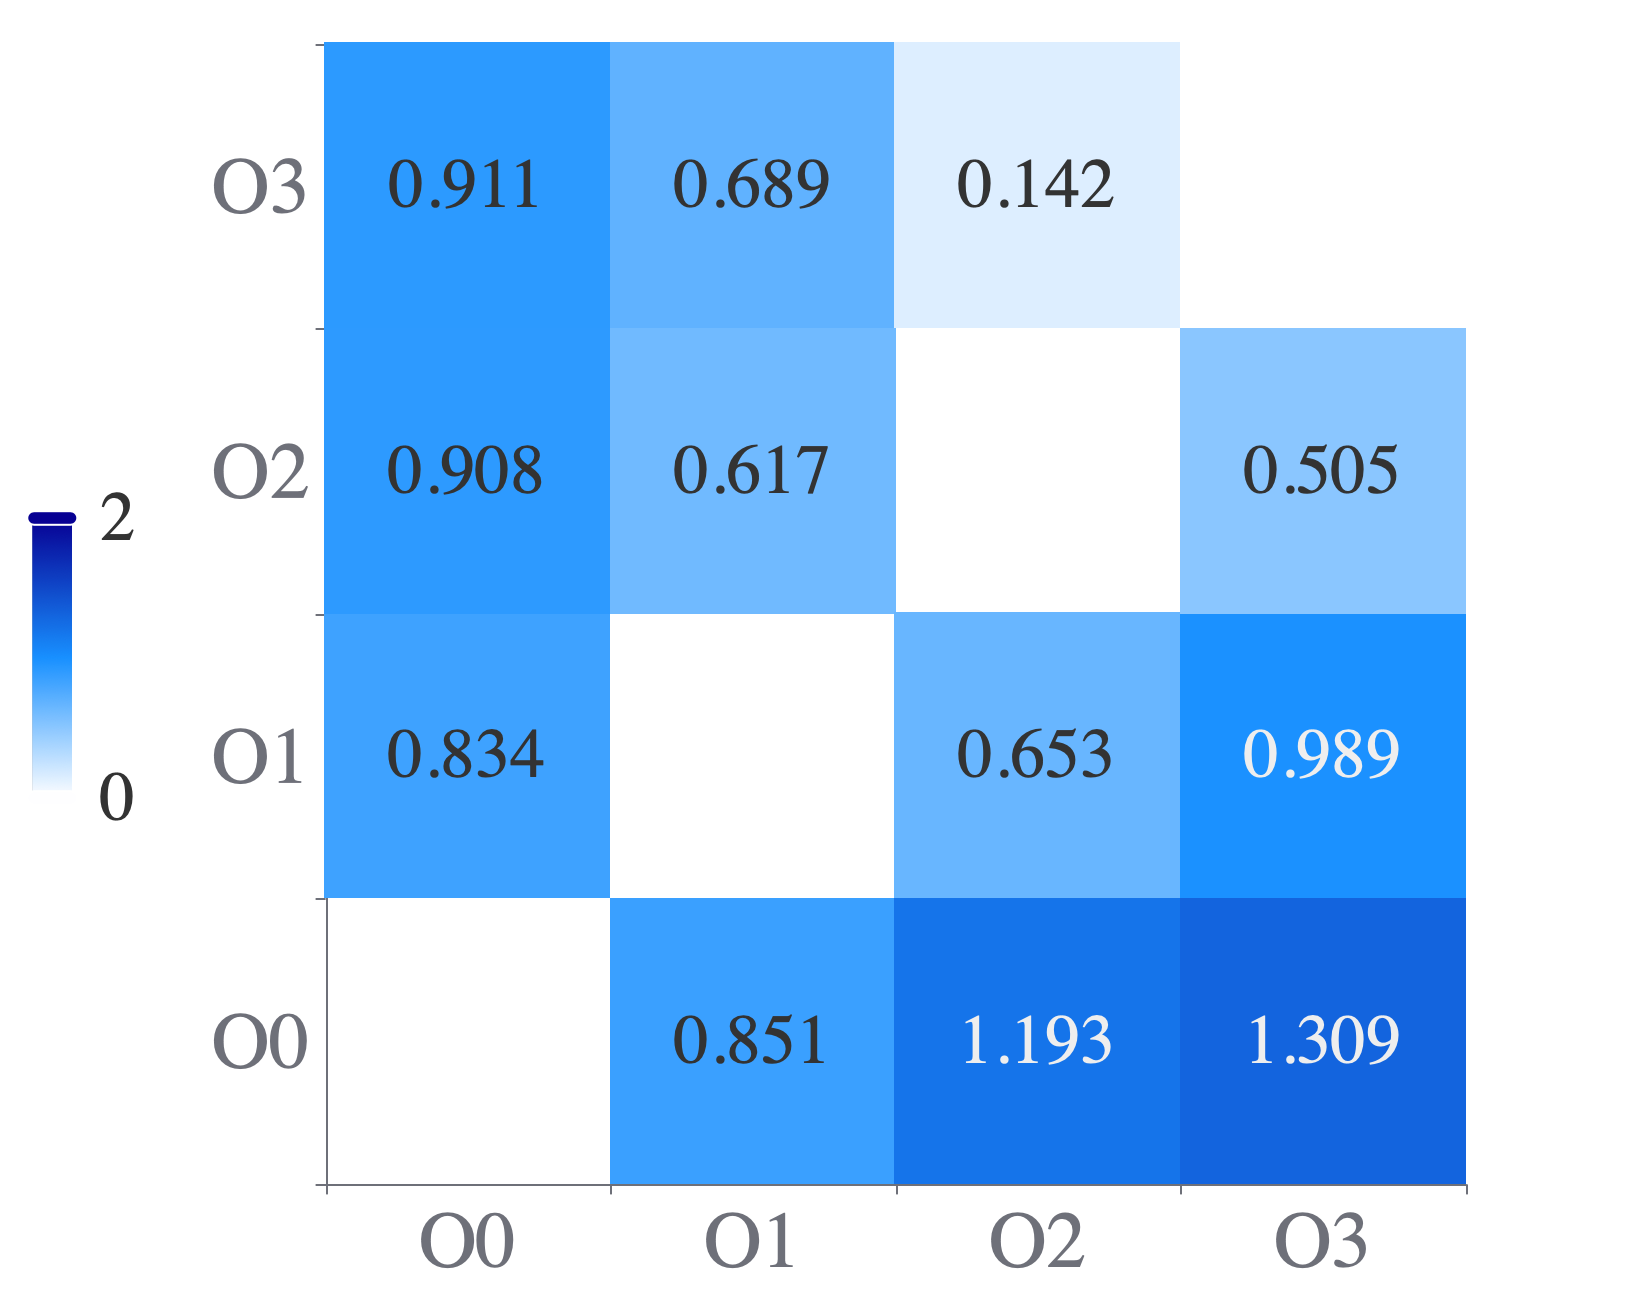}}
            \subfloat[assembly_difference-x64]{
                \label{same-arch-assembly-distribution-x64} 
                \includegraphics[width=0.24\textwidth]{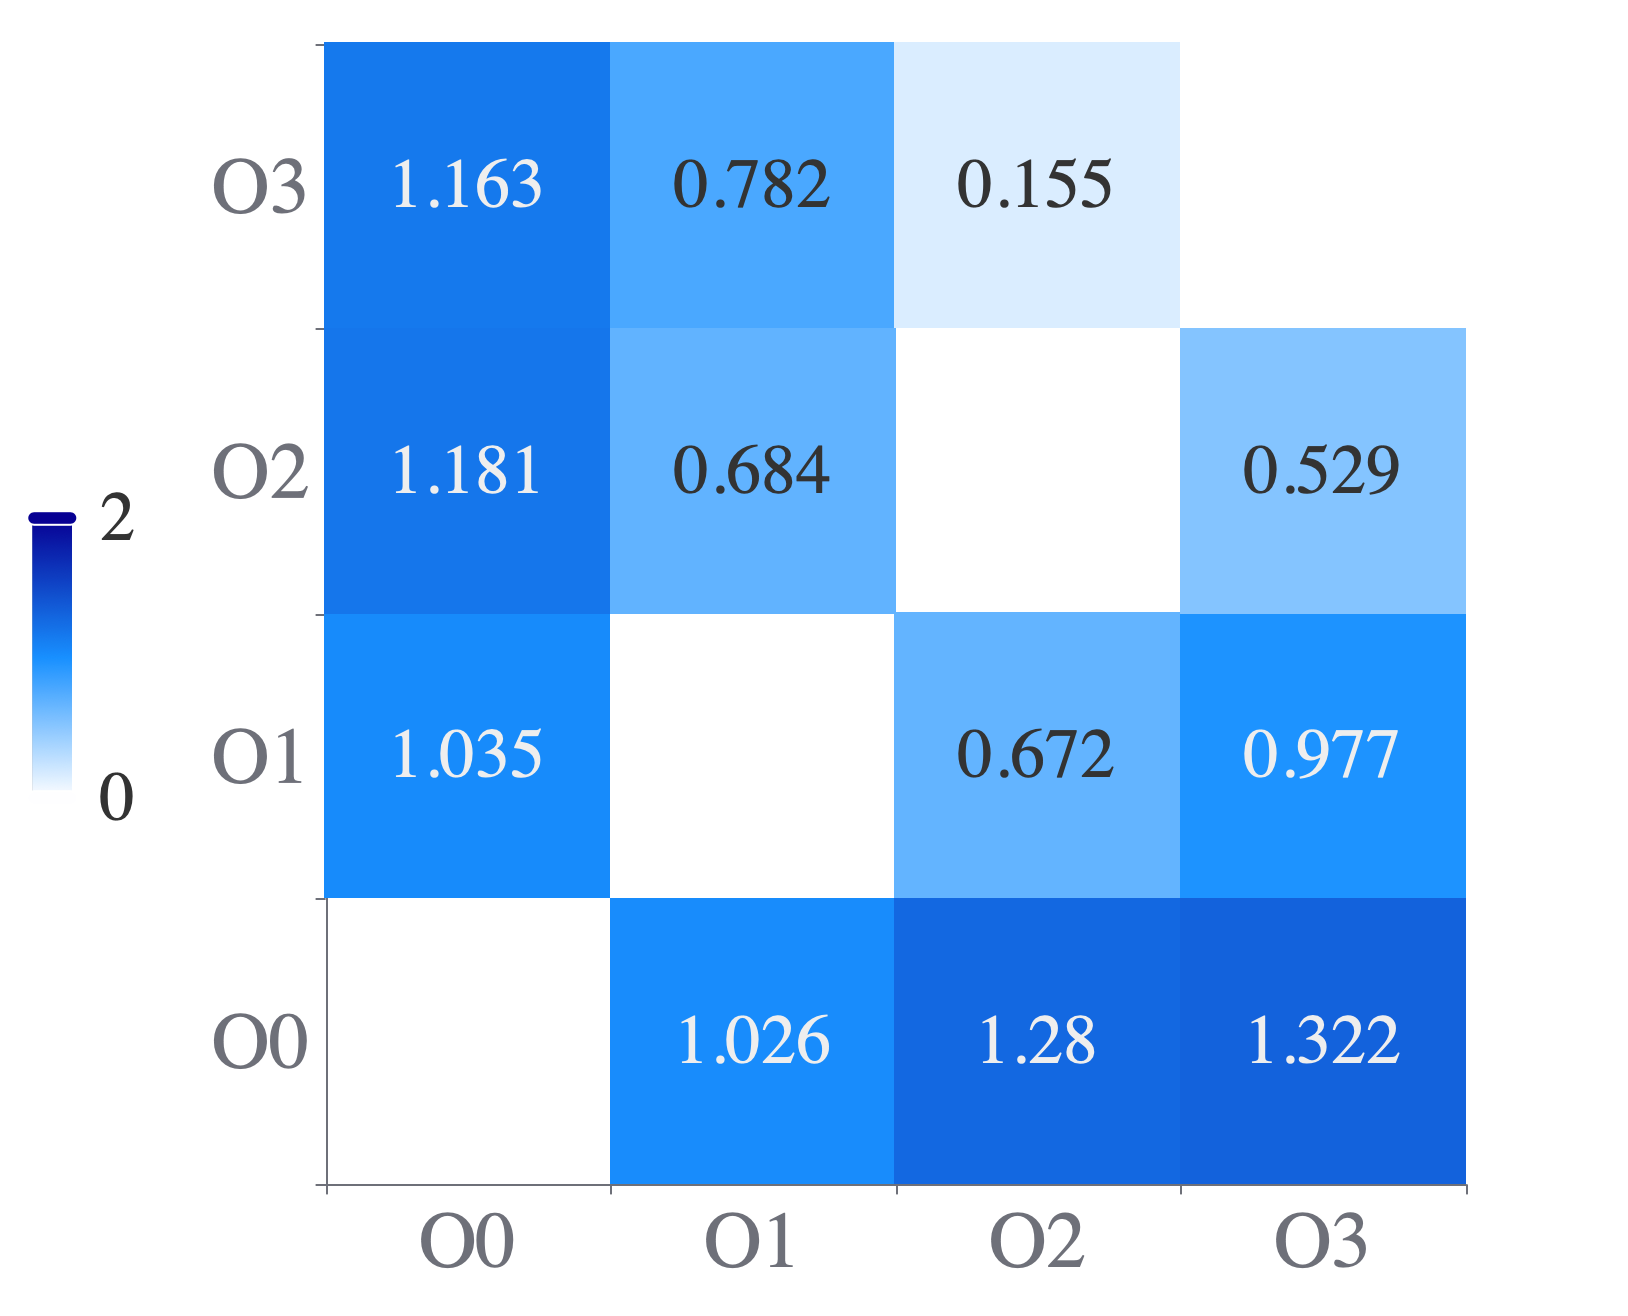}}
            \subfloat[AST_difference-x64]{
                \label{same-arch-V-ast-x64} 
                \includegraphics[width=0.24\textwidth]{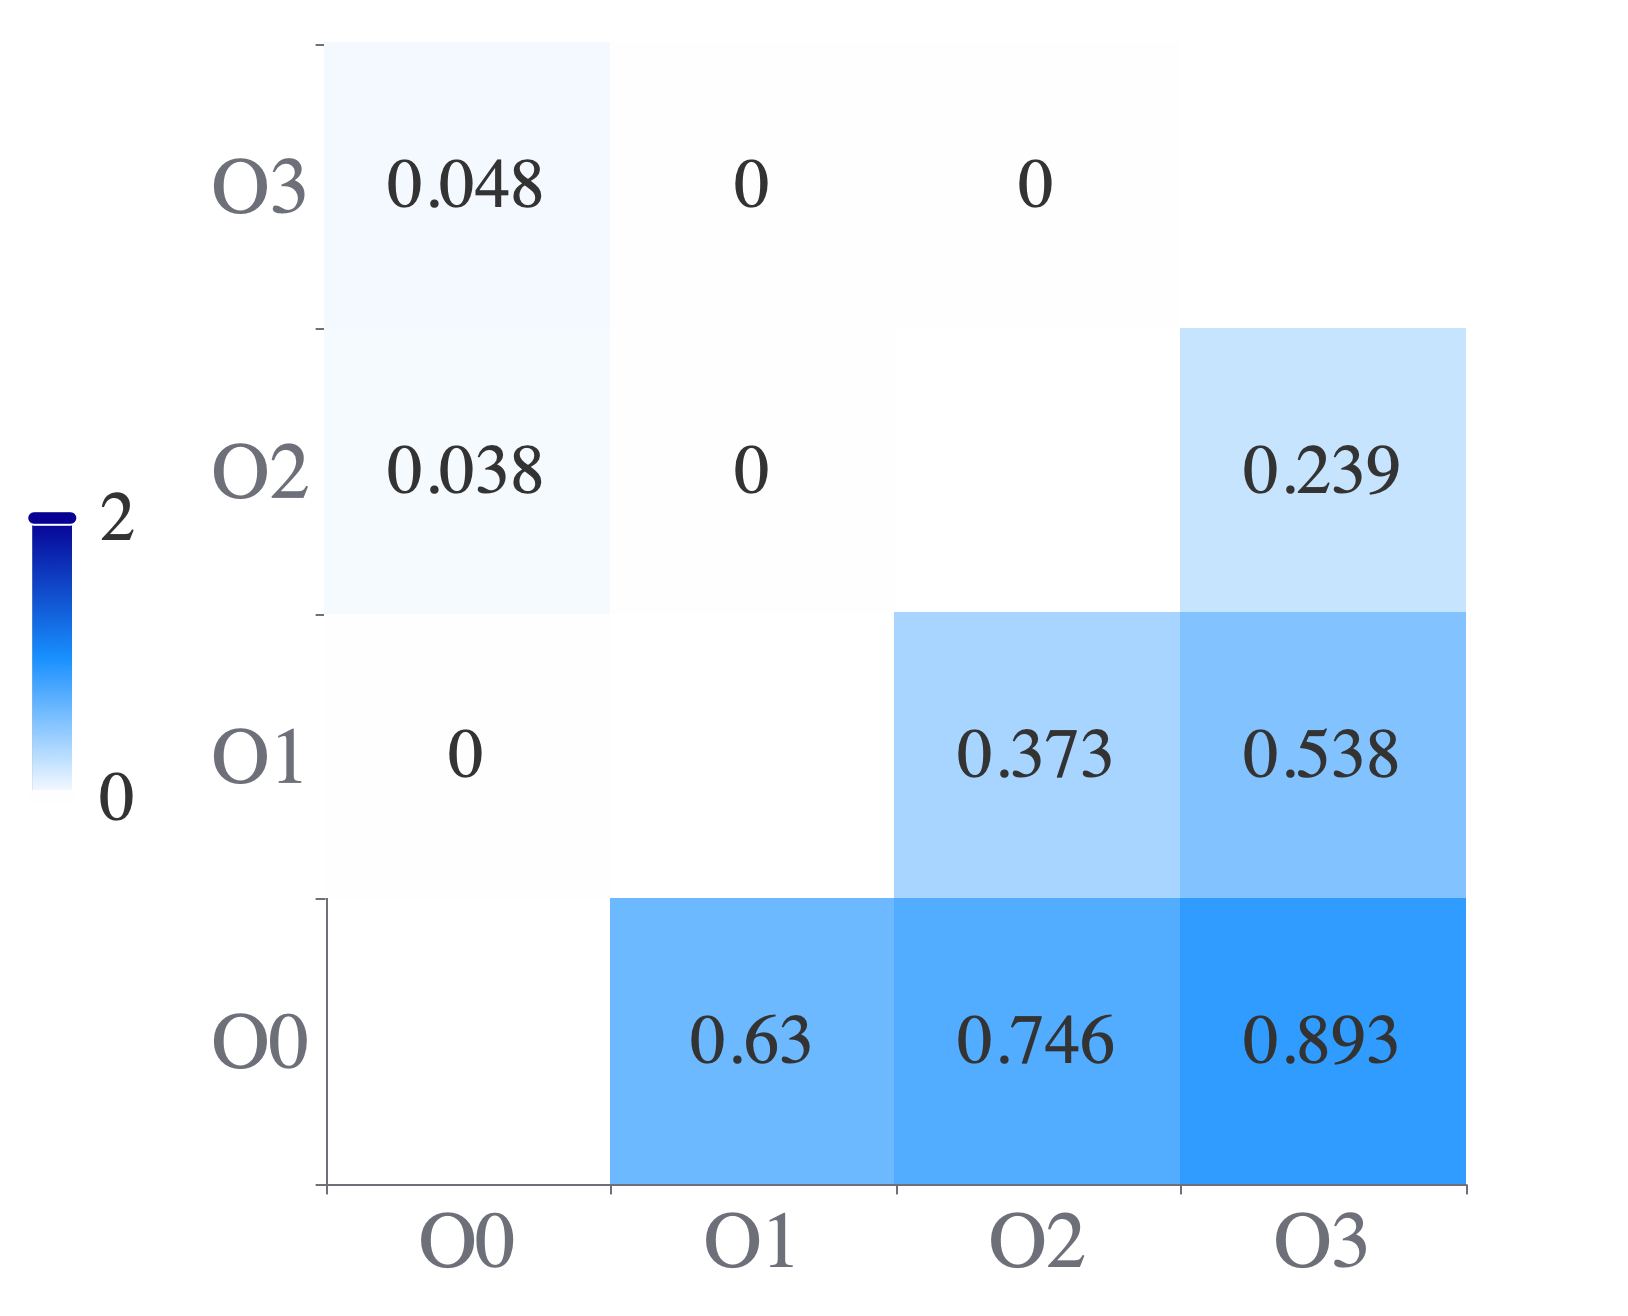}}
            \subfloat[CFG_difference-x64]{
                \label{same-arch-V-distribution-x64} 
                \includegraphics[width=0.24\textwidth]{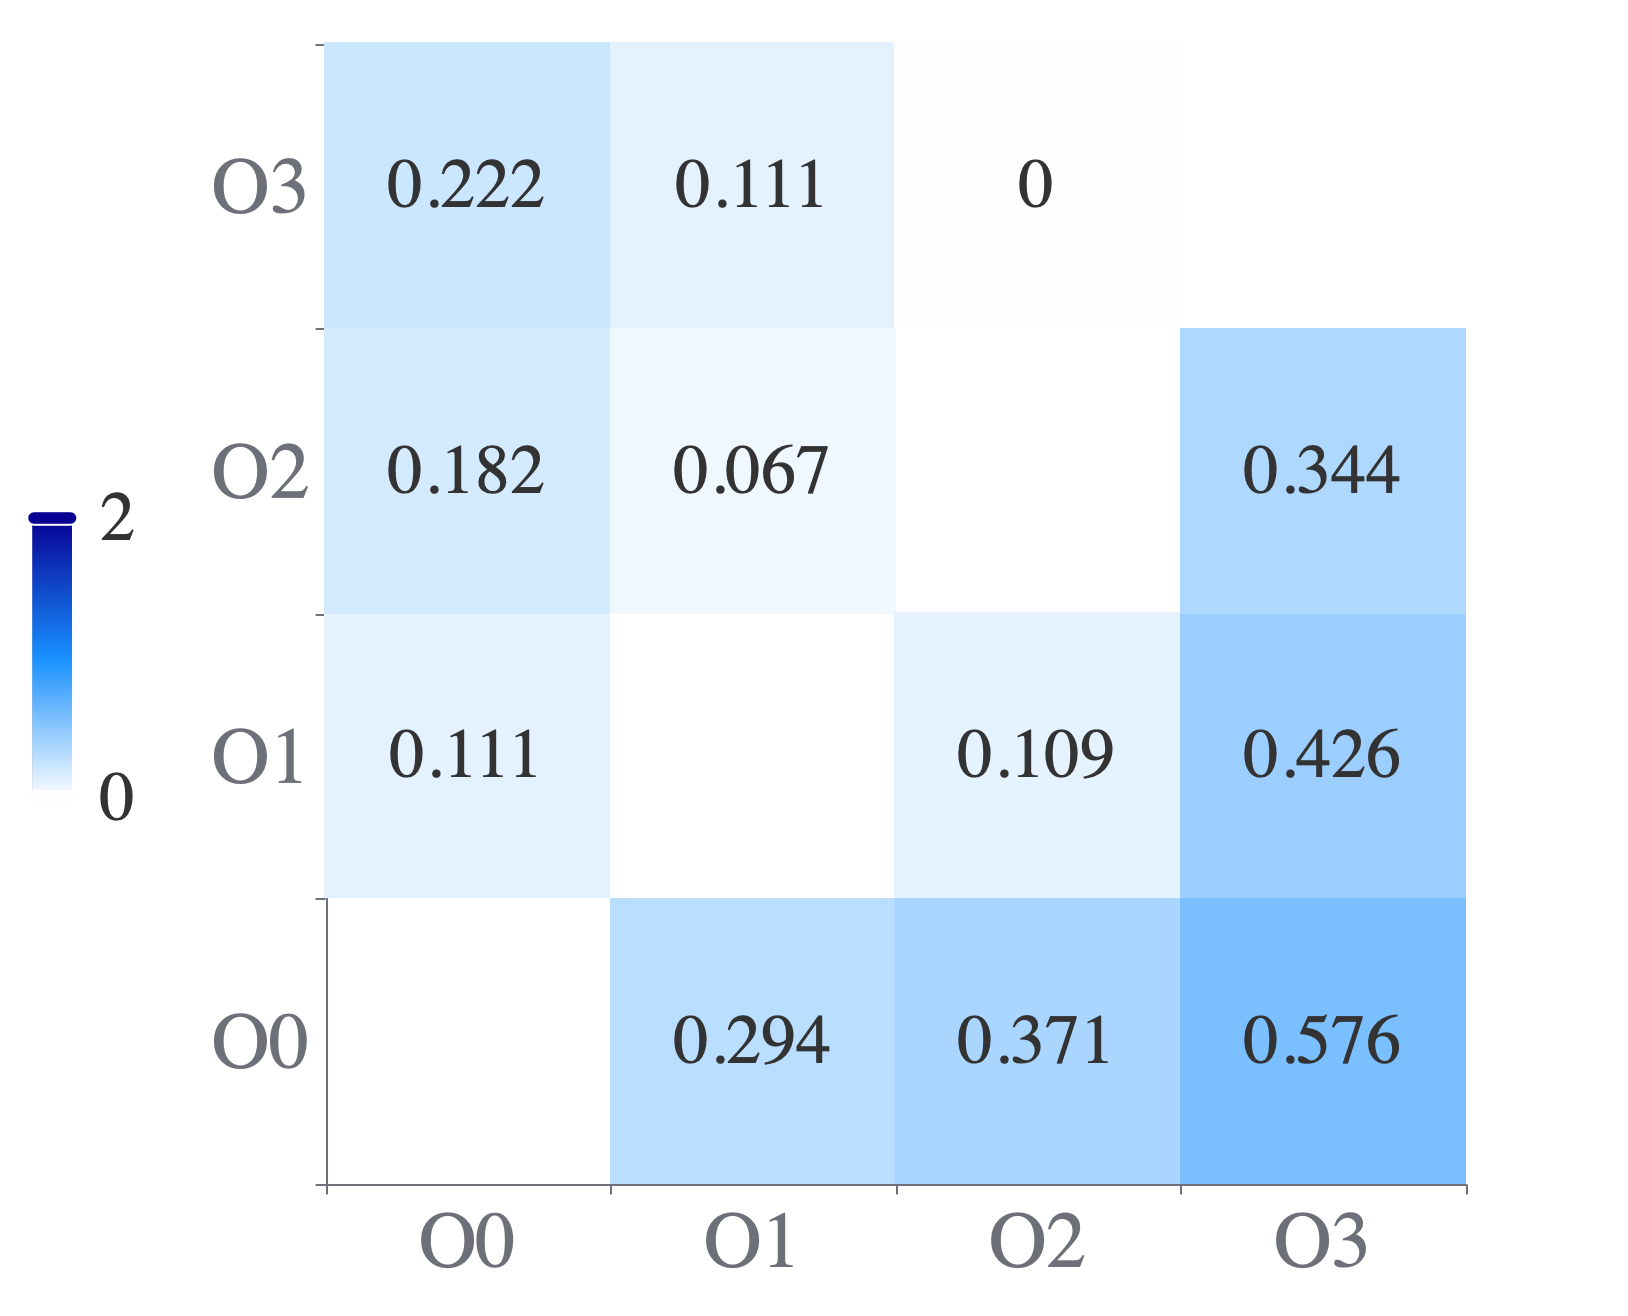}}

            \subfloat[rawbyte_difference-O2]{
                    \label{same-opt-rawbyte-distribution-O2} 
                    \includegraphics[width=0.24\textwidth]{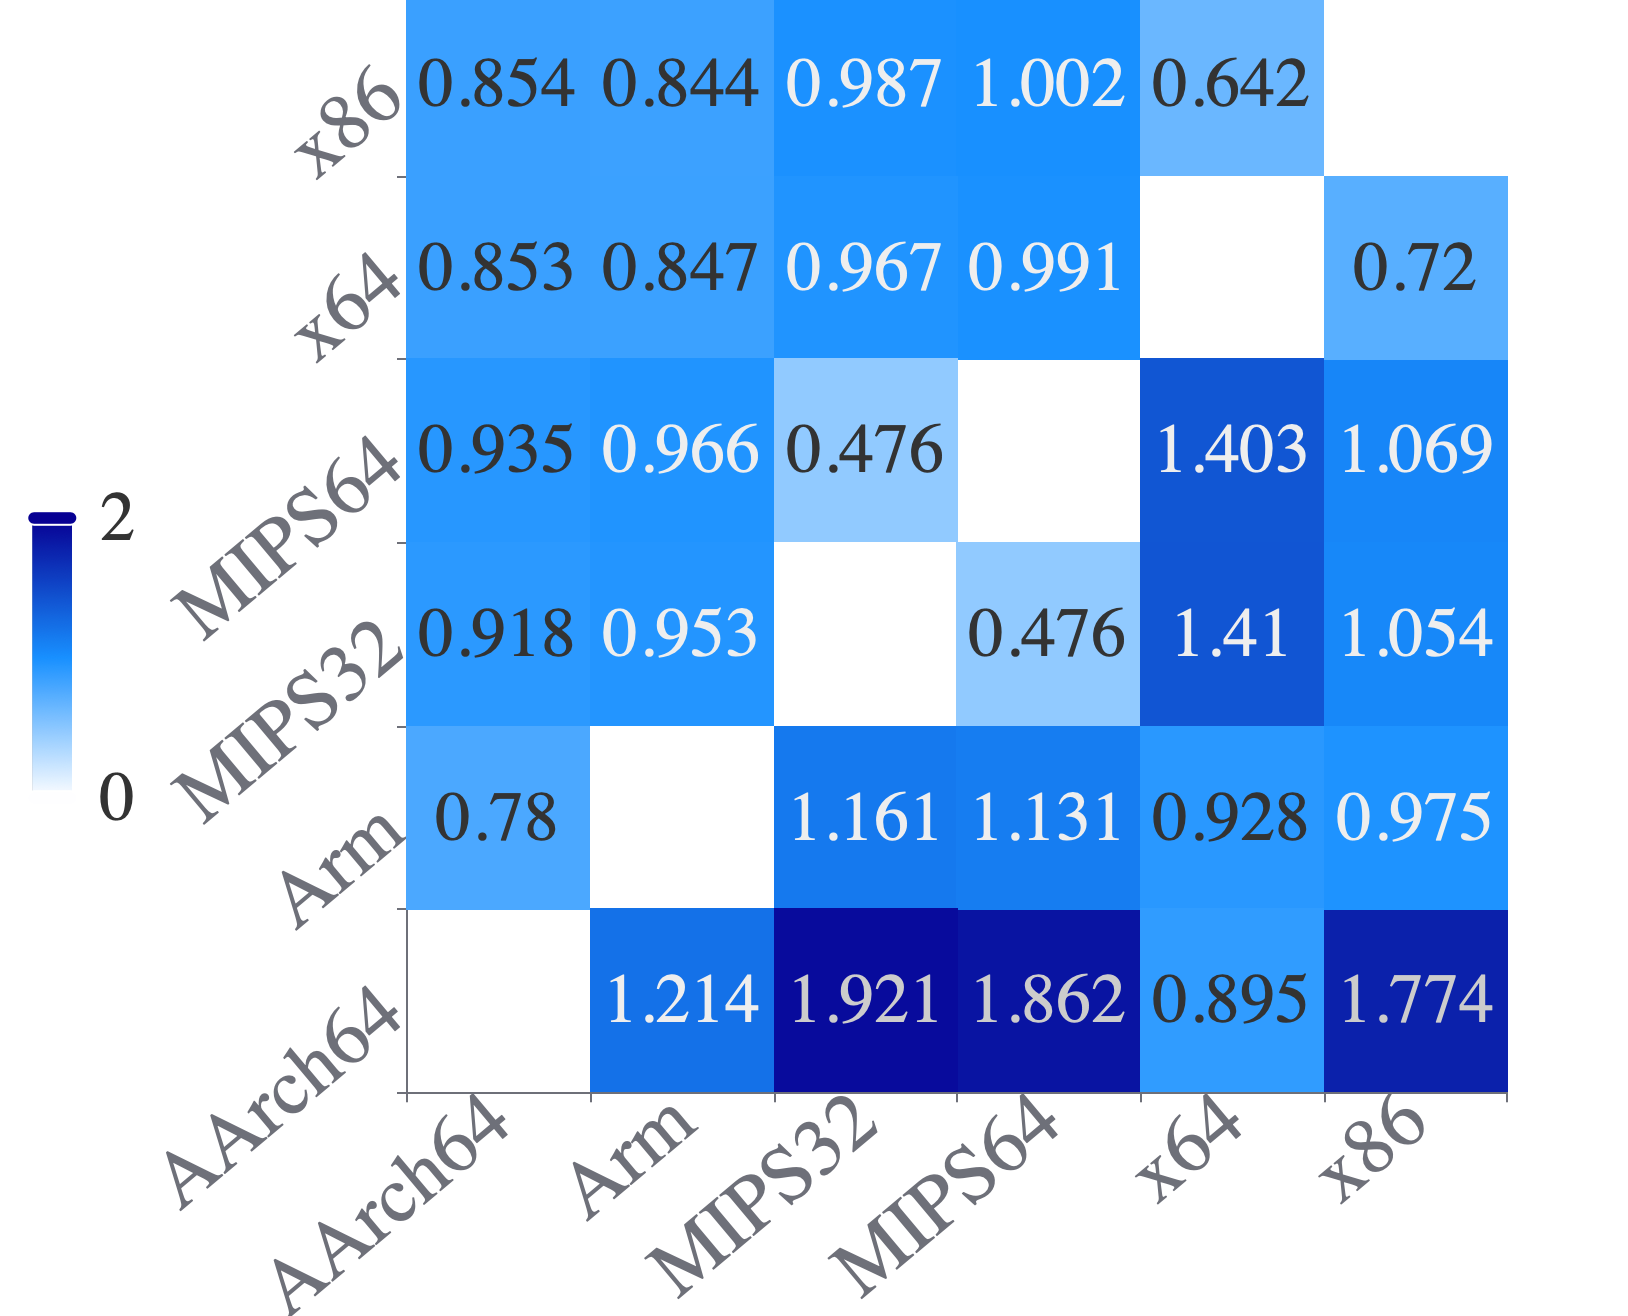}}
            \subfloat[assembly_difference-O2]{
                \label{same-opt-assembly-distribution-O2} 
                \includegraphics[width=0.24\textwidth]{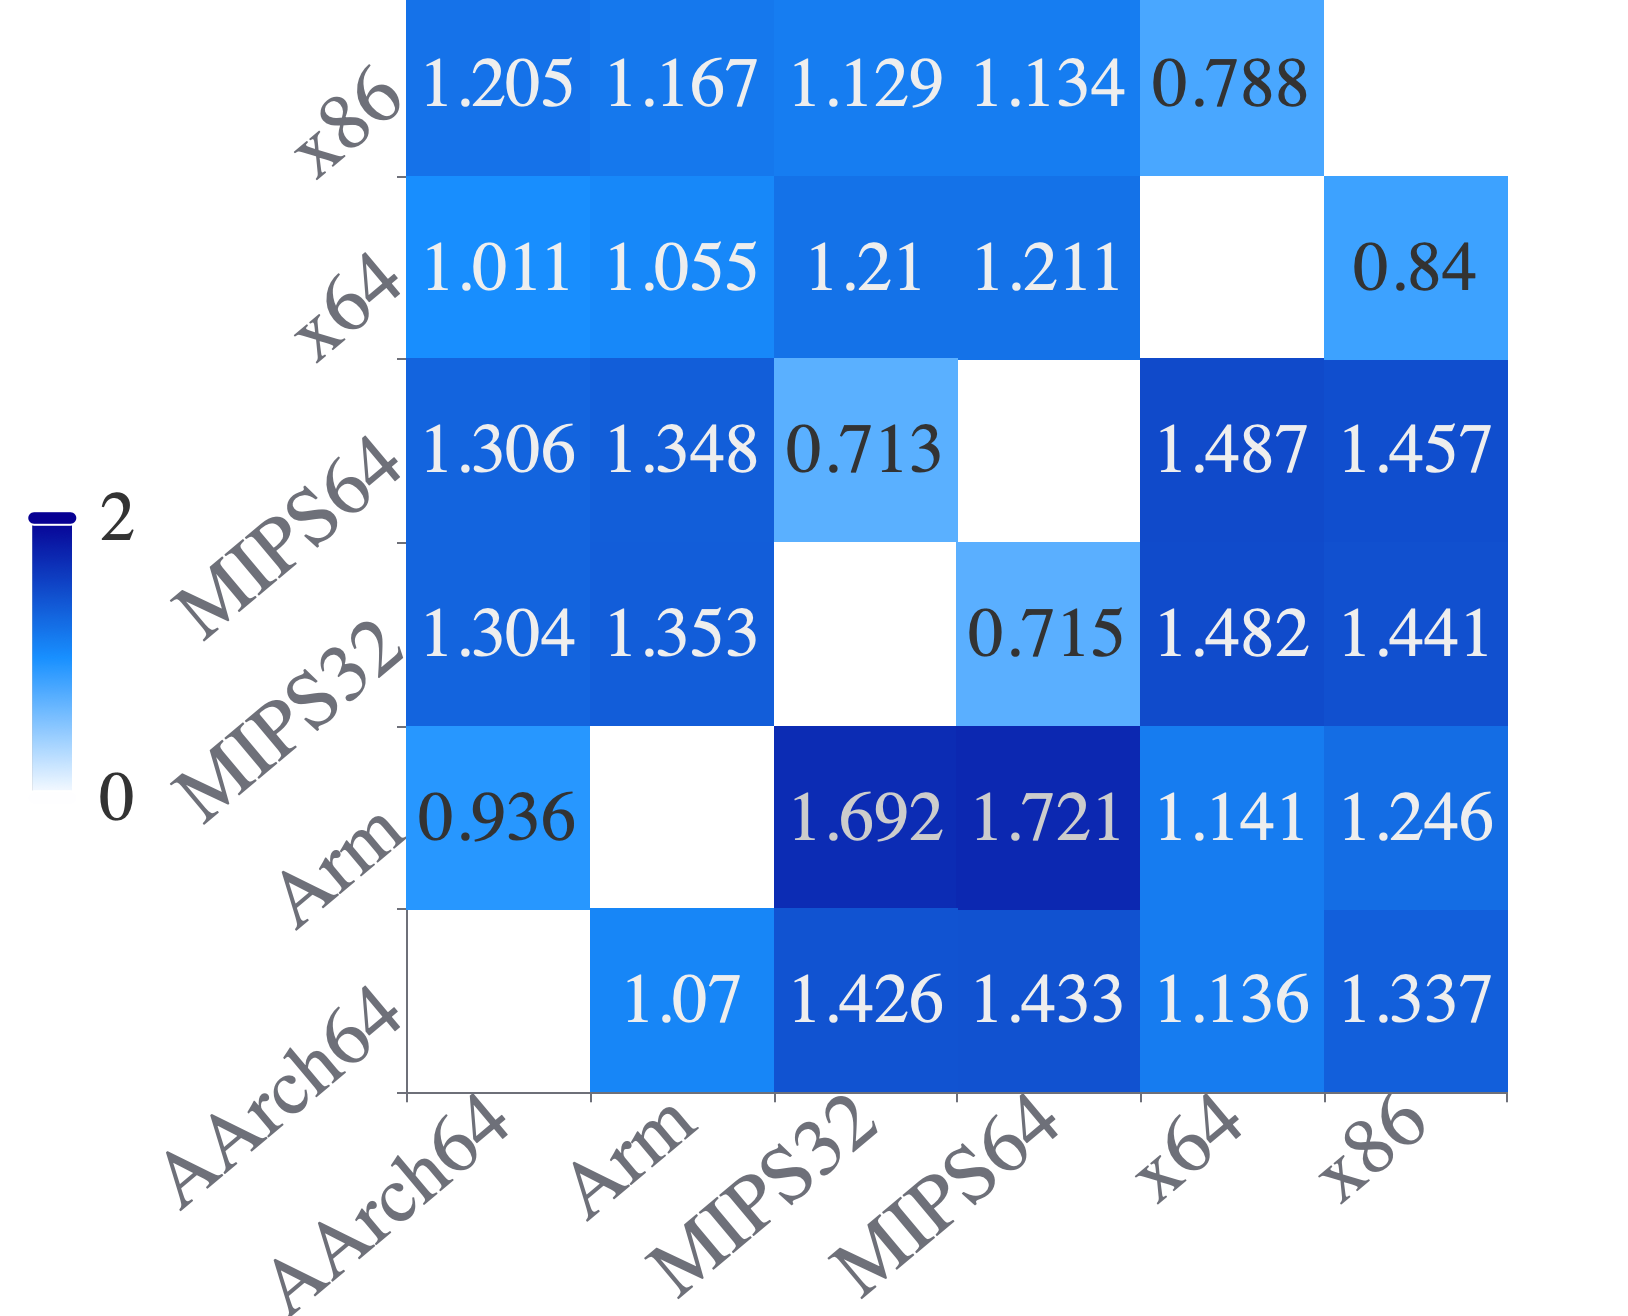}}
            \subfloat[AST_difference-O2]{
                \label{same-opt-V-ast-O2} 
                \includegraphics[width=0.24\textwidth]{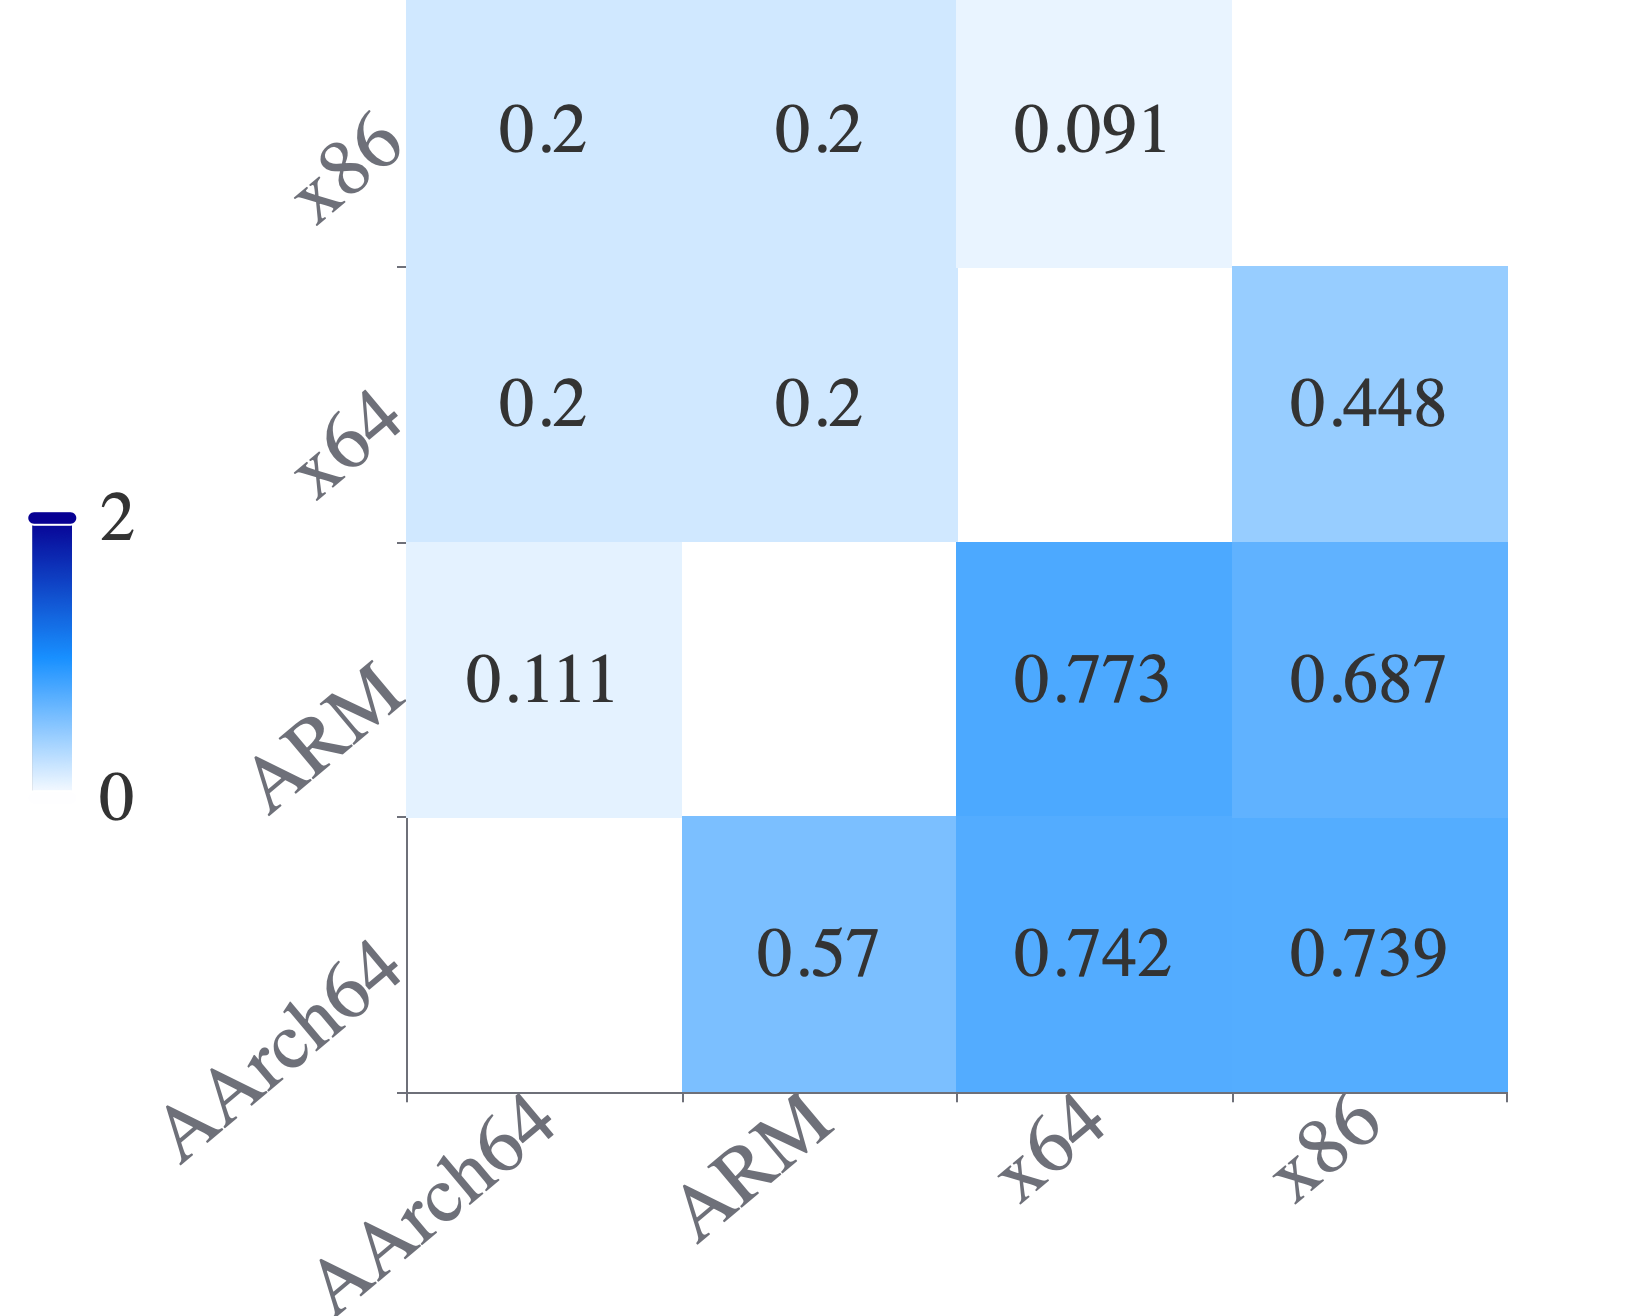}}
            \subfloat[CFG_difference-O2]{
                \label{same-opt-V-distribution-O2} 
                \includegraphics[width=0.24\textwidth]{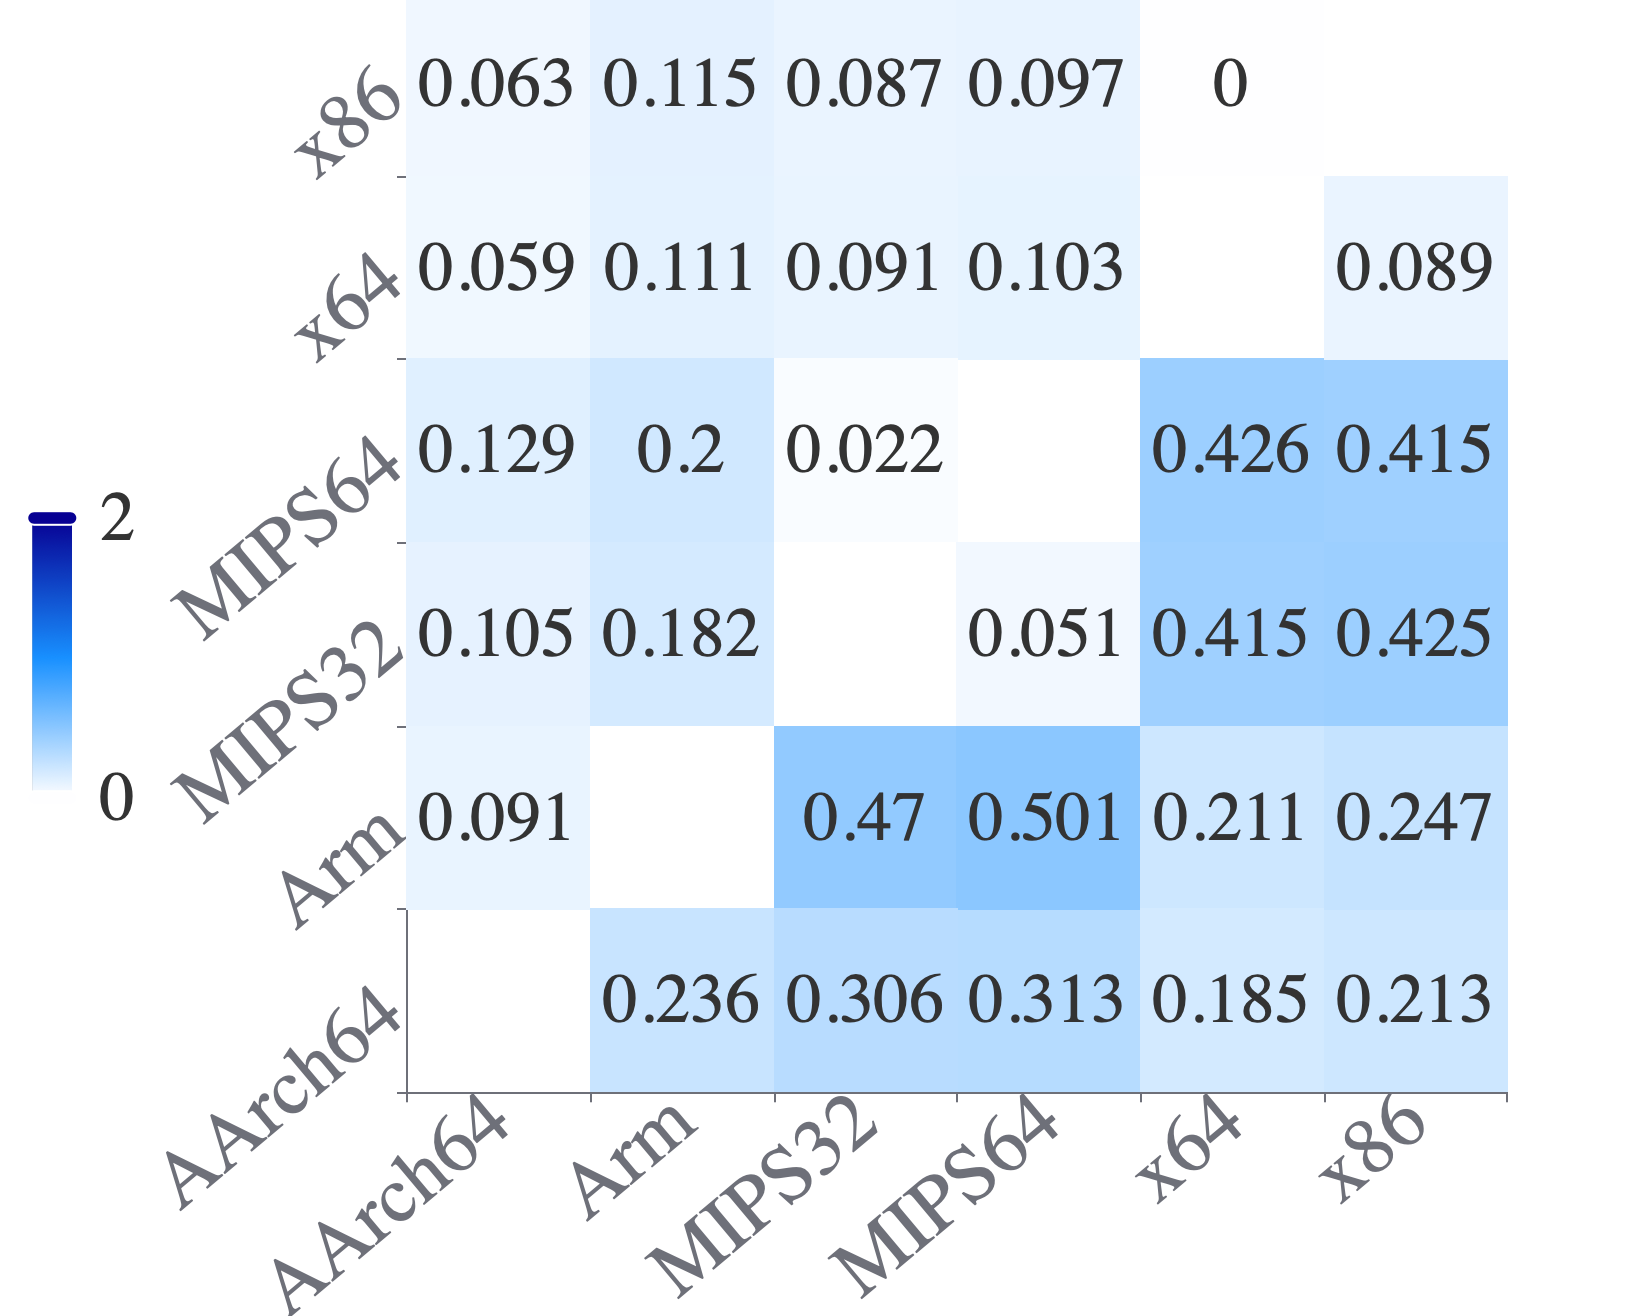}}

            \subfloat[rawbyte_difference-x64-O2]{
                    \label{same-opt-rawbyte-distribution-x64-O2} 
                    \includegraphics[width=0.24\textwidth]{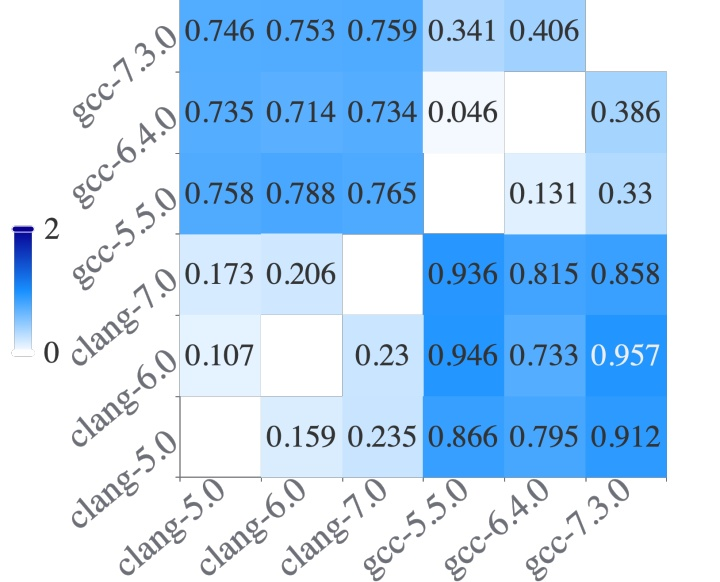}}
            \subfloat[assembly_difference-x64-O2]{
                \label{same-opt-assembly-distribution-x64-O2} 
                \includegraphics[width=0.24\textwidth]{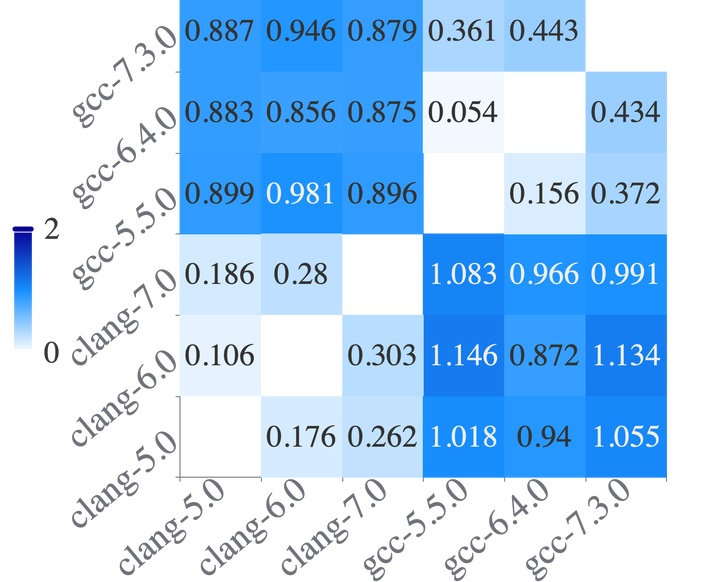}}
            \subfloat[AST_difference-x64-O2]{
                \label{same-opt-V-ast-x64-O2} 
                \includegraphics[width=0.24\textwidth]{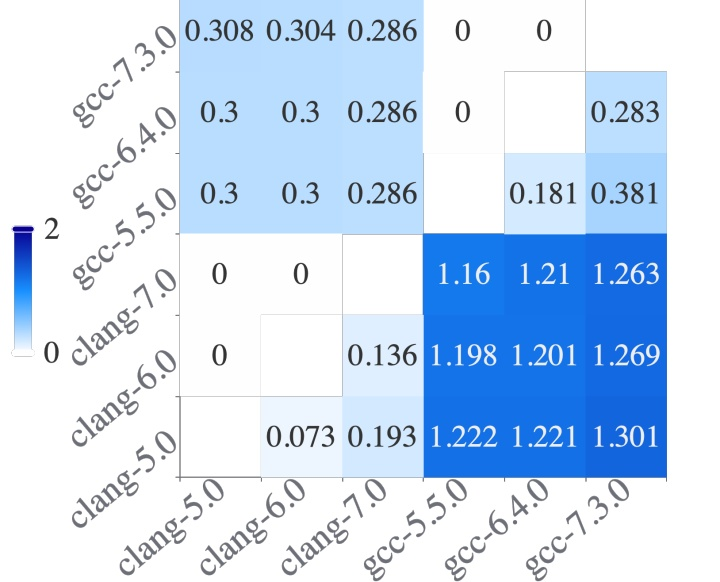}}
            \subfloat[CFG_difference-x64-O2]{
                \label{same-opt-V-distribution-x64-O2} 
                \includegraphics[width=0.24\textwidth]{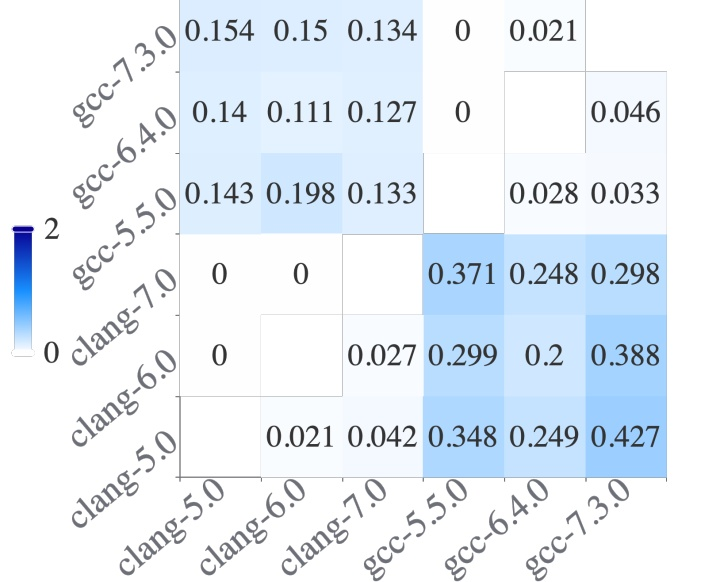}}
    \end{minipage}
    \caption{The difference between binary functions compiled with different optimization levels, architectures, and compilers. (a) and (b) are the string editing distance of the raw bytes and assembly code of functions compiled with -O0 - O3 optimization levels under x64, respectively. (c) and (d) are the relative difference in the count of vertices of abstract syntax tree (AST) and CFG. The upper left and down right values of each figure are the median and average values of the difference of all function pairs, respectively.}
    \label{fig:comparision-across-different-architectures}
\end{figure*}

\begin{figure*}[htbp]
    \begin{minipage}[t]{0.32\linewidth}
        \centering
            \subfloat[coreutils-nproc]{
                \label{fig1a} 
                \includegraphics[width=0.49\linewidth]{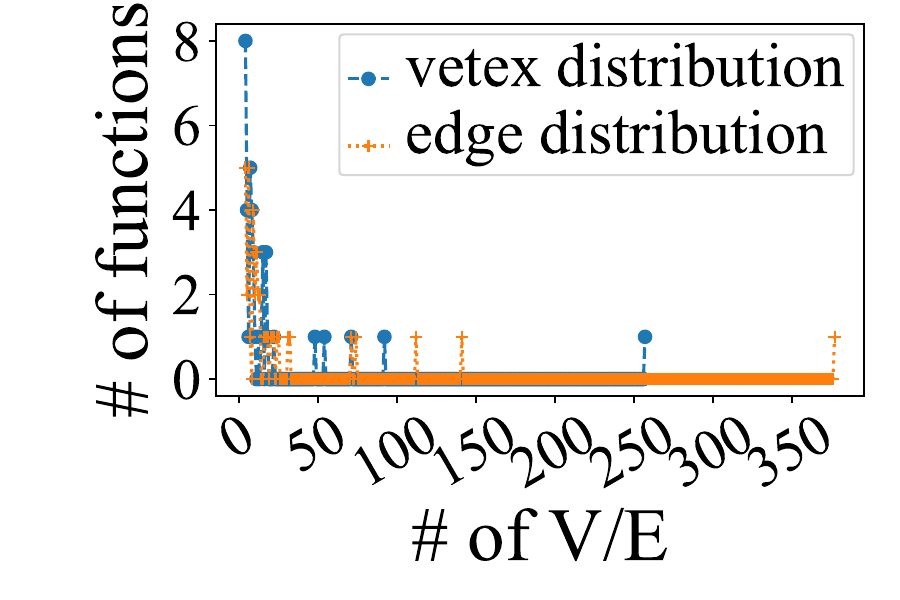}}
            \subfloat[findutils-frcode]{
                \label{fig1b} 
                \includegraphics[width=0.49\linewidth]{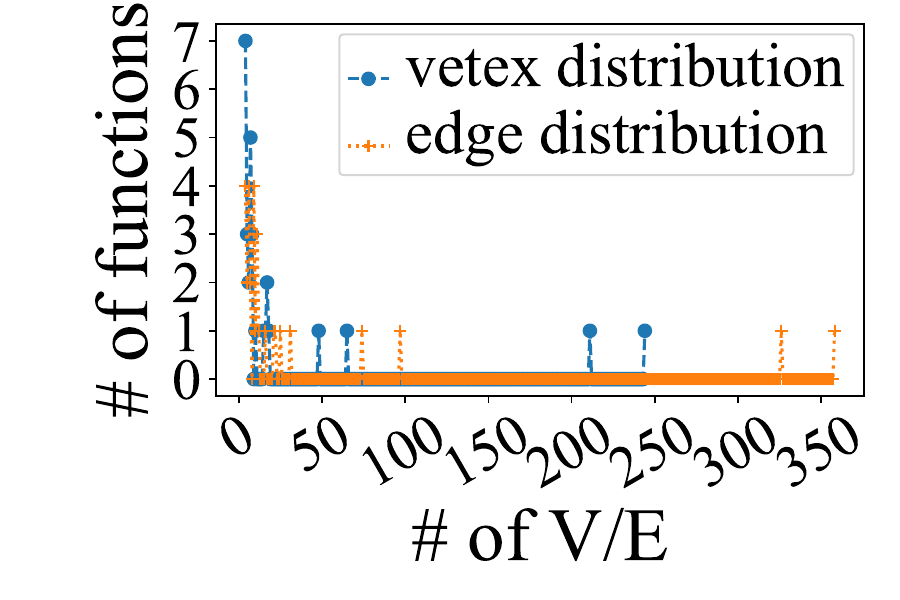}}
            \vfill
            \subfloat[inetutils-dns*]{
                \label{fig1c} 
                \includegraphics[width=0.49\linewidth]{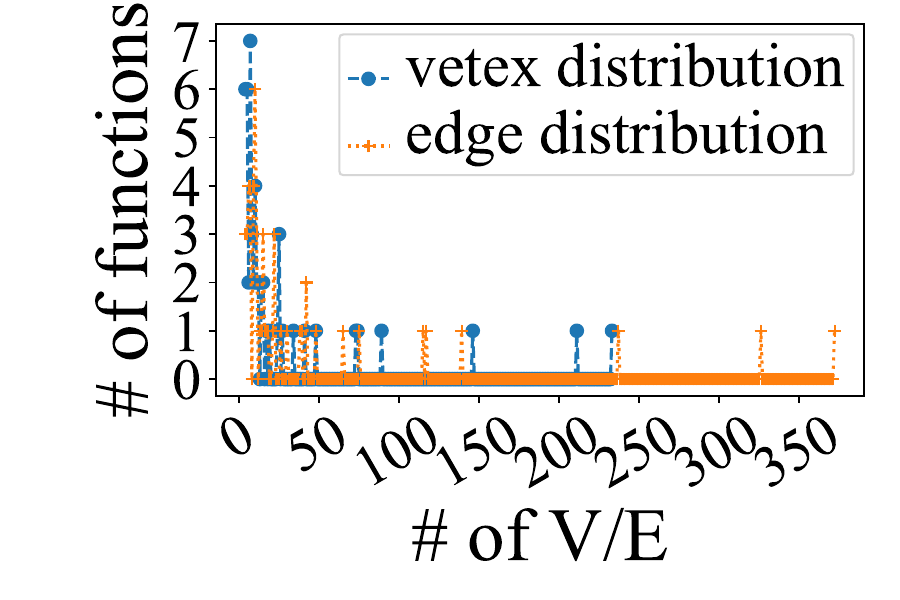}}
            \subfloat[inetutils-rexec]{
                \label{fig1d} 
                \includegraphics[width=0.49\linewidth]{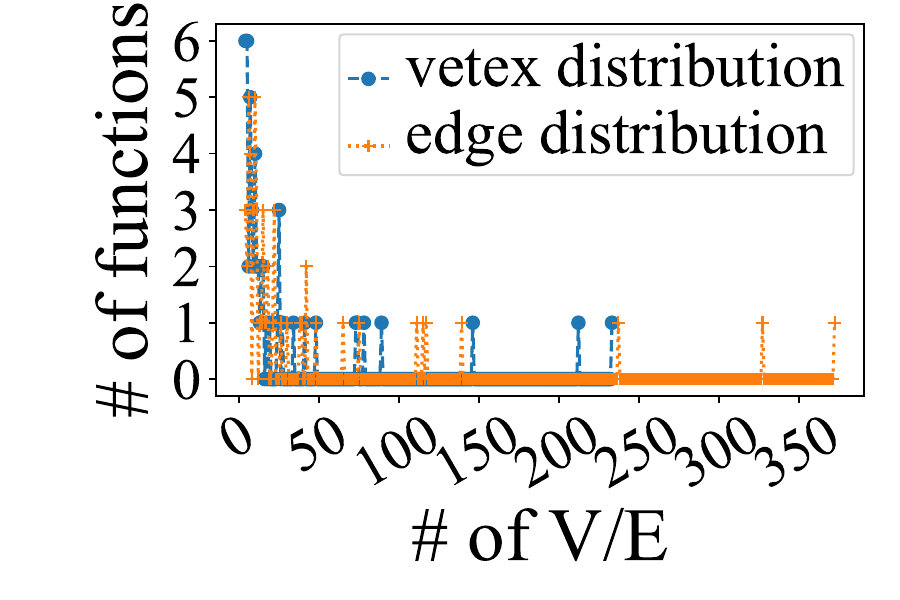}}
            \caption{The distribution of basic blocks and edges.}
            \label{fig:subfig1}
    \end{minipage}
\hfill
    \begin{minipage}[t]{0.32\linewidth}
        \centering
            \subfloat[coreutils-nproc]{
                \label{fig2a} 
                \includegraphics[width=0.49\linewidth]{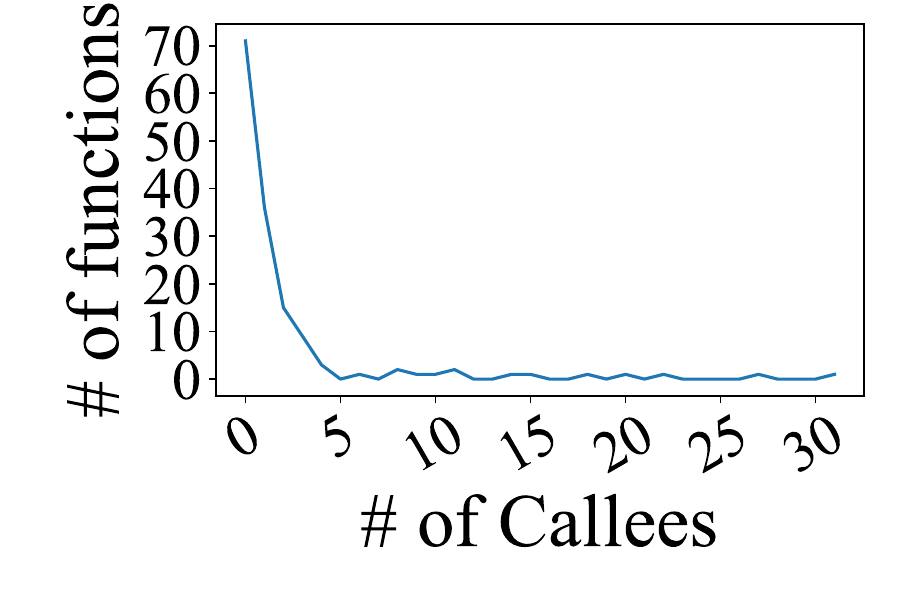}}
            \subfloat[findutils-frcode]{
                \label{fig2b} 
                \includegraphics[width=0.49\linewidth]{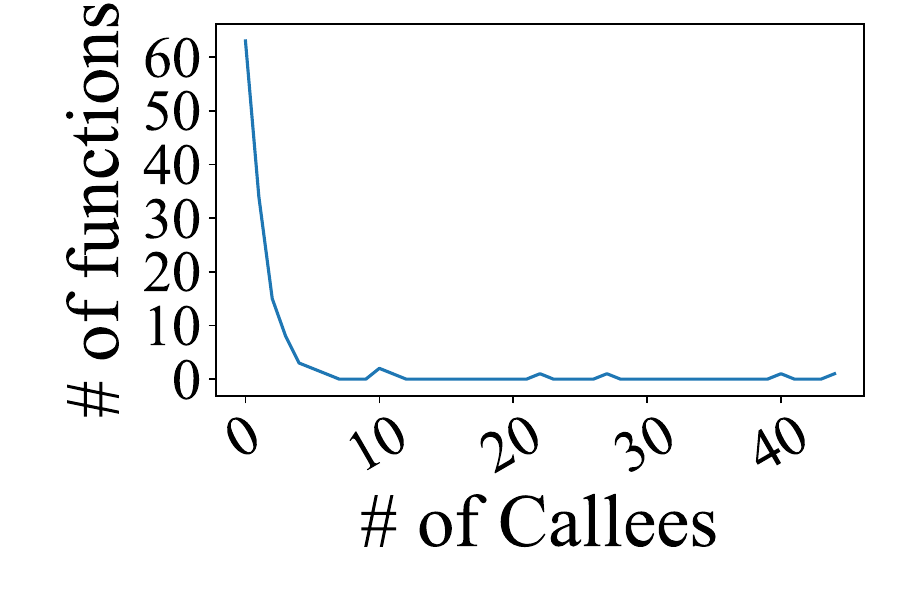}}
            \vfill
            \subfloat[inetutils-dns*]{
                \label{fig2c} 
                \includegraphics[width=0.49\linewidth]{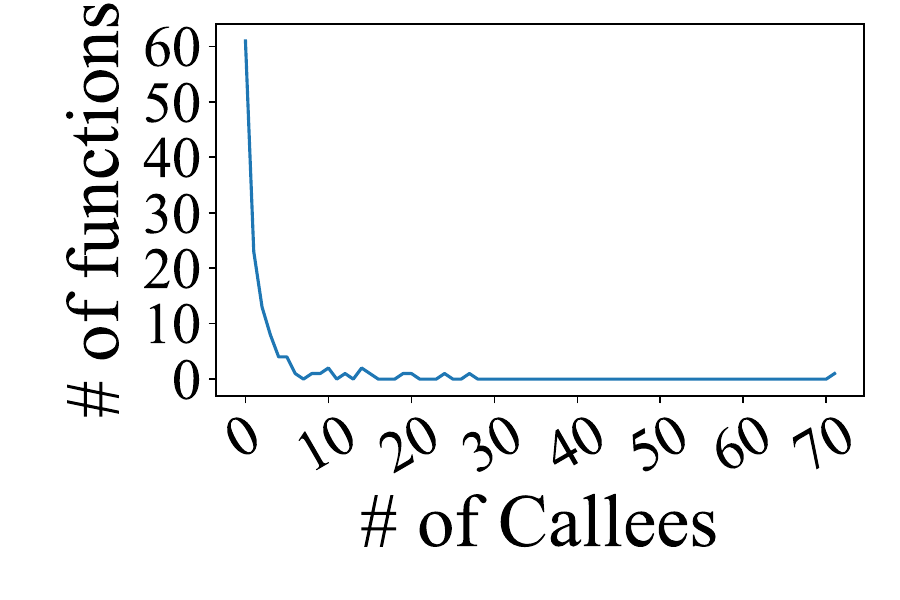}}
            \subfloat[inetutils-rexec]{
                \label{fig2d} 
                \includegraphics[width=0.49\linewidth]{fig/binary_selection/coreutils_coreutils-8.29_gcc-6.4.0_x86_64_O1_nproc.elf_funcCalls.pdf}}
            \caption{The distribution of FuncCalls.}
            \label{fig:subfig2}
    \end{minipage}
\hfill
    \begin{minipage}[t]{0.32\linewidth}
        \centering
            \subfloat[coreutils-nproc]{
                \label{fig3a} 
                \includegraphics[width=0.49\linewidth]{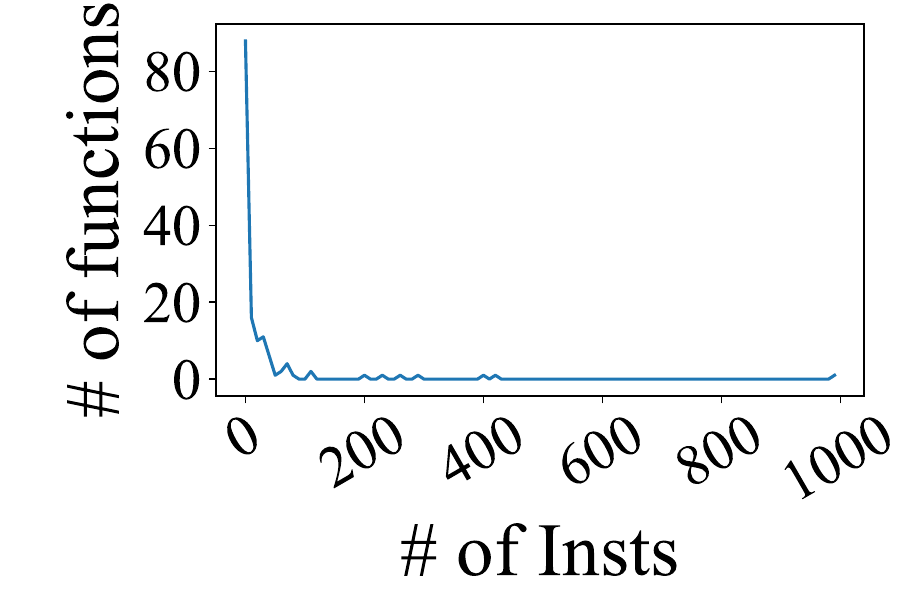}}
            \subfloat[findutils-frcode]{
                \label{fig3b} 
                \includegraphics[width=0.49\linewidth]{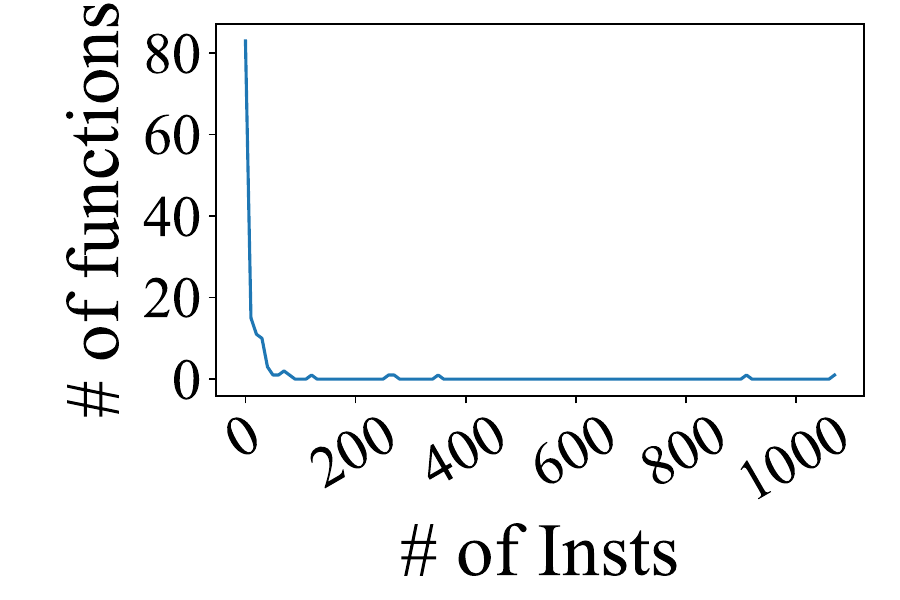}}
            \vfill
            \subfloat[inetutils-dns*]{
                \label{fig3c} 
                \includegraphics[width=0.49\linewidth]{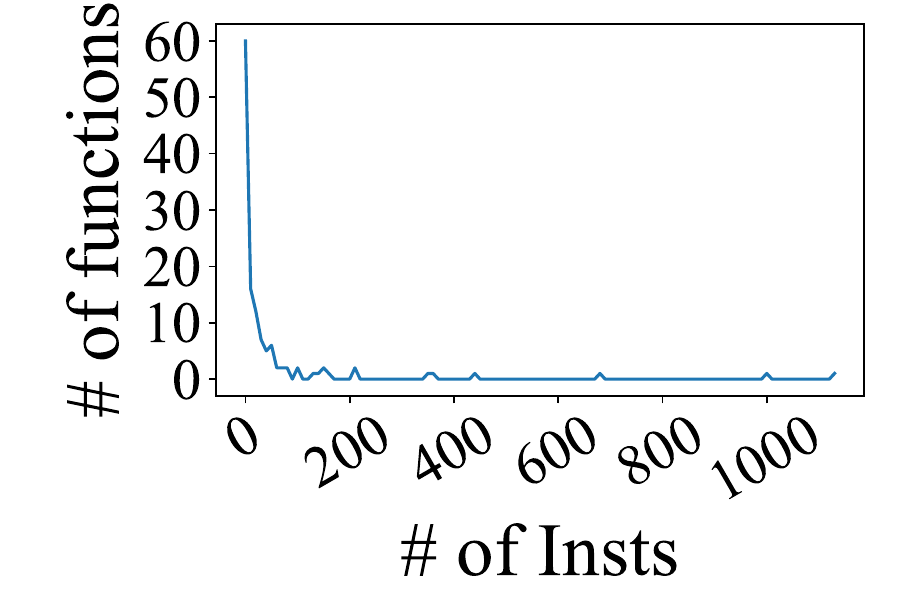}}
            \subfloat[inetutils-rexec]{
                \label{fig3d} 
                \includegraphics[width=0.49\linewidth]{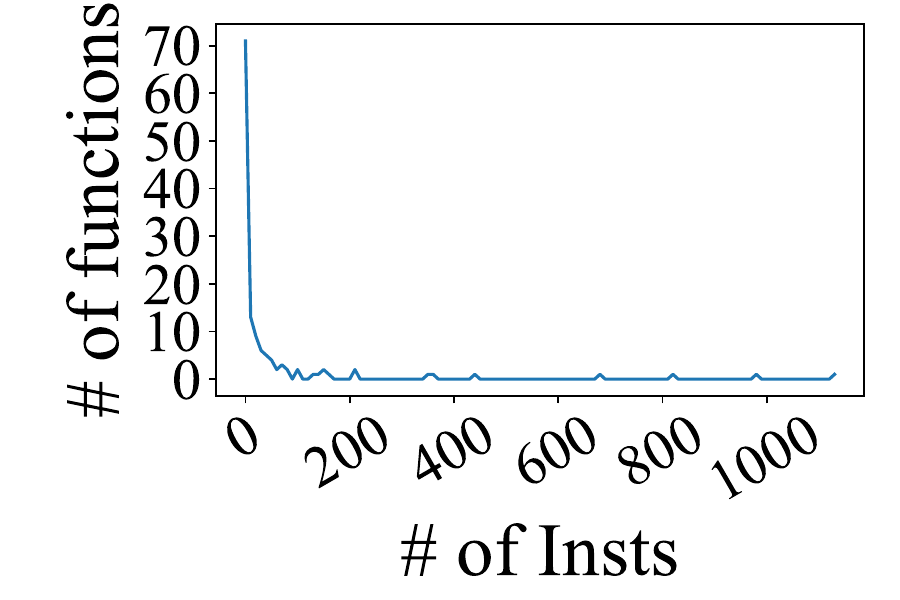}}
            \caption{The distribution of FuncSize.}
            \label{fig:subfig3}
    \end{minipage}
\end{figure*}

\begin{table*}[htbp]
    % \footnotesize
    \color{\tablecolor}
	\centering
	\caption{Basic-dataset.}
	\label{tab:software}\vspace{-6pt}
        \resizebox{0.82\linewidth}{!}
 	{
	\begin{tabular}{llllll}
		\toprule
		\textbf{\shortstack{Function}}   & \textbf{\shortstack{Program}}  & \textbf{\shortstack{\# of ELFs}} & \textbf{\shortstack{\# of funcs under ARM}}& \textbf{\shortstack{\# of funcs under x86}}& \textbf{\shortstack{\# of funcs under x64}}  \\
		\midrule
\rcolor		Calendars Calculating  & gcal-4.1   &2 &5,240&3,145&3,125\\% &  \\
%\rcolor		Database & recutils-1.7 &1&5,398&&\\%& \\
	     & gzip-1.9 &1&3,948&3,771&3,687\\%&   \\
		\multirow{-2}{*}{Data Compressing} & zstd-1.1.3* &1&6,055&8,220&8,064\\%&   \\
\rcolor		Data Encryption & OpenSSL-1.0.1f &3&207,120&206,520&177,153\\%& \\
		 & ccd2cue-0.5 &1&1,428&1,380&1,344\\%&   \\
	    \multirow{-2}{*}{File Converting}	 & enscript-1.6.6&1&1,644&1,524&1,488 \\%&   \\
\rcolor		File Objects Copying & xorriso-1.4.8 &1&12,215&12,067&12,042\\%&   \\
		File System & direvent-5.1 &1&21,256&7,875&16,713\\%&   \\
\rcolor		Graph Plotting   & plotutils-2.6 &2&946&858&834\\%&   \\
%		Kernel & vmlinux* & 4.1.52 &  \\
\rcolor		Language Engine & lua-5.3.5* &1&450&519&471\\%& \\
		 & dap-3.10 &1&756&750&714\\%&   \\
		\multirow{-2}{*}{Math Operation} & gsl-2.5 &1&10,998&1,400&2,031\\%&   \\
\rcolor		 & libmicrohttpd-0.9.59&1&5,248 &5,176&5,056\\%& \\
\rcolor	    & ngix-1.17.0*&1& 1,728&1,725&1,719\\%&  \\
\rcolor		\multirow{-3}{*}{Network} & osip-5.0.0 &1&4,941&4,944&4,917\\%&  \\
		Numeric Calculation Library & gmp-6.1.2&1&8,722&8,538&8,646 \\%&   \\
\rcolor		OS assisting & gnudos-1.11.4 &2&2,259&2,151&2,127\\%&   \\
		PostScript Converting & a2ps-4.14 &2&9,344&9,030&8,980\\%&   \\
\rcolor		Text Encoding Converting & libiconv-1.15 &2&659&659&659\\%& \\
		 & gawk-4.2.1&1&14,826&9,570&9,540 \\%&   \\
		\multirow{-2}{*}{Text Processing} & sed-4.5&1&6,705&6,657&6,603 \\%&   \\
\rcolor		& coreutils-8.29&2&6,858&6,396&6,309 \\%&   \\
\rcolor		& Busybox-1.27.0&1&104,364 &195,528&117,054\\%&   \\
\rcolor		& findutils-4.6.0 &1&2,340&2,301&2,262\\%&   \\
\rcolor		\multirow{-4}{*}{Utility} & inetutils-1.9.4 &1&2,985&2,928&2,889\\%&   \\
       \midrule
	    \textbf{Total} &&{33}&{443,045}&{503,632}&{404,427}\\
		\bottomrule
	\end{tabular}
	}%\vspace{-10pt}
\end{table*}

\begin{table}[htbp]
    % \footnotesize
    \scriptsize
    \color{\tablecolor}
	\centering
	\caption{IoT firmware.}
	\label{tab:Iotfirmware}
	\setlength{\tabcolsep}{1.0mm} 
 	{
	\begin{tabular}{lll}
		\toprule
		\textbf{\shortstack{Firmware}}   &  \textbf{\shortstack{\# of ELFs}} & \textbf{\shortstack{\# of funcs}}  \\
		\midrule
		CAP1200v1_1.0.0_20170801-rel61314_up.bin&176&56,741\\
\rcolor		COM_T01F001_LM.1.6.18P12_sign2_TPL.TL-SC4171G.bin&97&19,573\\
		COM_T01F001_LM.1.6.18P7_TPL.TL-SC4171G.bin&96&19,242\\
\rcolor		COVR-2600R_FW101b05_0911_txbfdisable0911190427.bin&281&19,242\\
		COVR-2600R_FW101b05_beta01_hcr2.bin&284&75,435\\
\rcolor		COVR-3902_ROUTER_v101b05.bin&284&75,435\\

	DAP2610-firmware-v101-rc017.bin&128&52,222\\
\rcolor			DLINK_DNR-322.2.10b022.10.0612.2014.bin&236&150,757\\
	DLINK_DNR-322L.1.40b011.16.1219.2012.bin&225&130,155\\
\rcolor			Dap2610-firmware-v101-beta28-rc0480306165616.bin&128&52,246\\
		\midrule
		Sum &1,935&651,048\\
		\bottomrule
	\end{tabular}
	}
\end{table}

\subsection{Evaluation Dataset}
\label{sub:evaluationdataset}
As discussed in~\autoref{sub:eval-dataset}, basic-dataset should contain representative benchmark programs with different function attributes. To construct the basic-dataset, in this paper, we first calculate the attribute distribution of BinKit~\cite{kim:tse:2022}. Then, we deduplicate the binaries with similar function attributes. Specifically, as shown in \autoref{fig:subfig1}, \autoref{fig:subfig2}, and \autoref{fig:subfig3}, the distribution of the number of basic blocks, callees, and assembly instructions are similar for the four presented binaries. Thus, we only keep one of them in the basic-dataset.  Finally, as shown in~\autoref{tab:software}, we select 25 open-source programs, including 33 ELFs and 1,351,104 functions, to construct the basic-dataset.  These 25 programs are compiled with four popular optimization levels (from O0 to O3) under three architectures ARM x86 and x64. We select these three ISAs because the architectures that existing \BCSD approaches support vary a lot. It is impractical to re-implement all the existing \BCSD approaches to support all the ISAs. Thus, we choose the ISAs supported by over half of the  \BCSD approaches in ~\autoref{tab:BCSD-comparision}.
In the application-dataset, the ten IoT firmware images, which
include 1,935 ELFs and 651,048 functions is shown in~\autoref{tab:Iotfirmware}. 

\subsection{Binary Comparison}
\label{sub:binarychange}
We perform a comprehensive binary diffing to understand the binary change of 100,000 binary function pairs that are compiled with various compiler options. Specifically,  we measure binary changes from four aspects (which can present prevalent code representations.), including the raw byte change, assembly change, and the change of the number of nodes of the AST and CFG across architectures, optimization levels, and toolchains. When performing cross-ISA and cross-compiler comparisons, we randomly set the optimization levels to -O2. When performing the cross-optimization level comparison, we randomly set the ISA to x64. As shown in~\autoref{fig:comparision-across-different-architectures}, we find that compared to raw byte, assembly code, and AST, the graph representation of binary code is more suitable for the \BCSD problem since CFG is more stable across-architectures, optimization levels, and compilers, i.e., the median and average values of the difference of all function is smallest in the CFG comparison, which benefits the embedding networks to generate similar code embeddings for functions compiled from the same source code.

\subsection{Vulnerable Function Confirmation}
\label{sub:vulnerableFunctionConfirm}
Actually, vulnerability confirmation contains two phrases---rough match and precise comparison. In the rough match, researchers identify the semantically similar functions that are highly likely compiled from the same source code of the queried vulnerabilities in a large function repository (such as IoT devices). In the precise comparison, researchers need to determine whether the semantically similar functions are buggy by performing accurate patch presence tests~\cite{jiang2020pdiff,zhang2018precise}.  
For most \BCSD approaches listed in~\autoref{tab:BCSD-comparision}, including Gemini~\cite{xu2017neural}, VulSeeker~\cite{gao2018vulseeker}, SAFE~\cite{massarelli2018safe}, and Oscar~\cite{peng2021could}, they are essentially seeking the same affected functions in the search repository. Namely, \BCSD is used to perform a rough match. Consequently, using state-of-the-art AI-powered \BCSD approaches, the search results obtained in~\autoref{subsub:VulnerabilitySearch} are potentially vulnerable functions. To finally examine the patch presence for these potentially vulnerable functions, one needs to generate and compare the summaries of specific patches' semantics.

In ~\autoref{subsub:VulnerabilitySearch},  we manually compare the pseudocode snippets (an ISA agnostic language similar to source code) of the search result and query function obtained by IDA pro to examine whether they are semantically identical. Specifically, we perform data flow analysis, constant string comparison, and call function comparison to determine whether two pseudocode snippets are compiled from the same source code.
